# Supplementary material for: Room Temperature Fiber-Coupled single-photon devices based on Colloidal Quantum Dots and SiV centers in Back Excited Nanoantennas
Source: arXiv:2303.10679 source file (2023-03-19)
Supplement: Supplementary file 1 [file AppendixD1.tex]

\section{Appendix D - Estimation of in-fiber collection efficiency}
The idea behind the calculation of the coupling efficiency is to calculate the fraction of the collected photons from all the emitted photons using back excitation. At first, we need to set a higher limit to the percentage of photons we may collect to the fiber at zero loss. To do that, we need to measure the K space image using the back excitation system. Collecting the emitted light with Olympus 0.9 NA objective and placing a K-space lens on the emission path, we may see on our CMOS camera the information about the momentum ($\vec{k_x}, \vec{k_y}$) distribution of the emitted photons bounded to 0.9 NA. Knowing the pixel size, one may calculate the exact circle that bound a specific NA (cone of angle $\theta_{NA}$). For our instance, it is necessary to measure the relative amount of the intensity that is bounded in the 0.22 NA (since that is the NA of the fiber) in a mathematical manner:
\begin{equation}
   \frac{\eta_{NA = 0.22}}{\eta_{NA = 0.9}} = \frac{ \int_{0}^{\theta_{NA = 0.22}}d\theta sin(\theta) \int_{0}^{2\pi} I(\theta,\phi)d\phi}{\int_{0}^{\theta_{NA = 0.9}}d\theta sin(\theta) \int_{0}^{2\pi} I(\theta,\phi) d\phi}
\end{equation}
Where $\eta$ is the collection efficiency and $I(\theta,\phi)$ is the intensity in the k-space image.
To calculate the collection efficiency as the function of the NA from the K space image, one mast integrates a cumulative integral over the whole k space image. We have found that :
\begin{equation}
   \eta_{NA = 0.22} = 0.32   \qquad  \eta_{NA = 0.9} = 0.91
\end{equation}
Hence the fraction would be 
\begin{equation}
    \frac{\eta_{NA = 0.22}}{\eta_{NA = 0.9}} = 0.3516 
\end{equation}
In other words, we found that $35.19 \% $  of the light collected by 0.9 NA objective can be confined into a cone of an angle $\theta_{NA = 0.22}$. Now, we need to get a measure of actual data to find the coupling efficiency. To do that, we will analyze the spectrum measurement and compare the counts we measured on the pixies spectrometer camera using a collection with a 0.22 NA fiber and a 0.9 NA objective.
\begin{equation}
    \frac{I_{Fiber\: Coupled}}{I_{0.9 NA\: objective}} = \frac{\int_{\lambda = 550 nm}^{\lambda = 700 nm} I_{Fiber\: Coupled}(\lambda) d\lambda \cdot \gamma_{Fiber}^{-1}}{\int_{\lambda = 550 nm}^{\lambda = 700 nm} I_{0.9 NA\: objective}(\lambda) d\lambda \cdot \gamma_{Objective}^{-1}}
    \label{equation:fiberc}
\end{equation}
where the integral represents the area under the spectrum and $\gamma$ stands for the loss in each system.

The losses in the objective system should be divided into 2 distinct types:
\begin{equation}
    \gamma_{objective} = \gamma_{system \: loses} \cdot \gamma_{spectrometer \: slit}
\end{equation}
Where $\gamma_{system \: loses}$ are the losses induced by the optical system itself (partial transmission of mirrors and filters) and $\gamma_{spectrometer \: slit}$ is the losses caused by the entrance slit of the spectrometer. Since the entrance slit of the spectrometer is slightly smaller than the whole emission spatial beam, the light that propagates into the slit is only a portion of the light that comes towards the slit.
To calculate the fraction of the transmitted light, we will use the following approach, assuming the beam is distributed like a Gaussian with a center in the middle of the slit (the system was aligned in such a manner), we may find the fraction of the light in a rectangular slit by using the following equation:
\begin{equation}
    \gamma_{spectrometer \: slit} = \frac{\Gamma w}{\pi \cdot \Gamma^2}
    \label{equation:slit}
\end{equation}
Where $\Gamma$ is the FWHM of the Gaussian on the spectrometer camera, and $w$ is the slit width. 
The FWHM of the power distribution was calculated by summing the intensities along the camera (and not along the grating). It may be seen in the figure below \ref{fig:pixel}  that the FWHM is 44 pixels.
\begin{figure} [H] % opens the figure environment. the '[H]' forces the image to be Here
    \centering % puts the image in the horizontal center of the page
    \includegraphics[width = 0.7\textwidth]{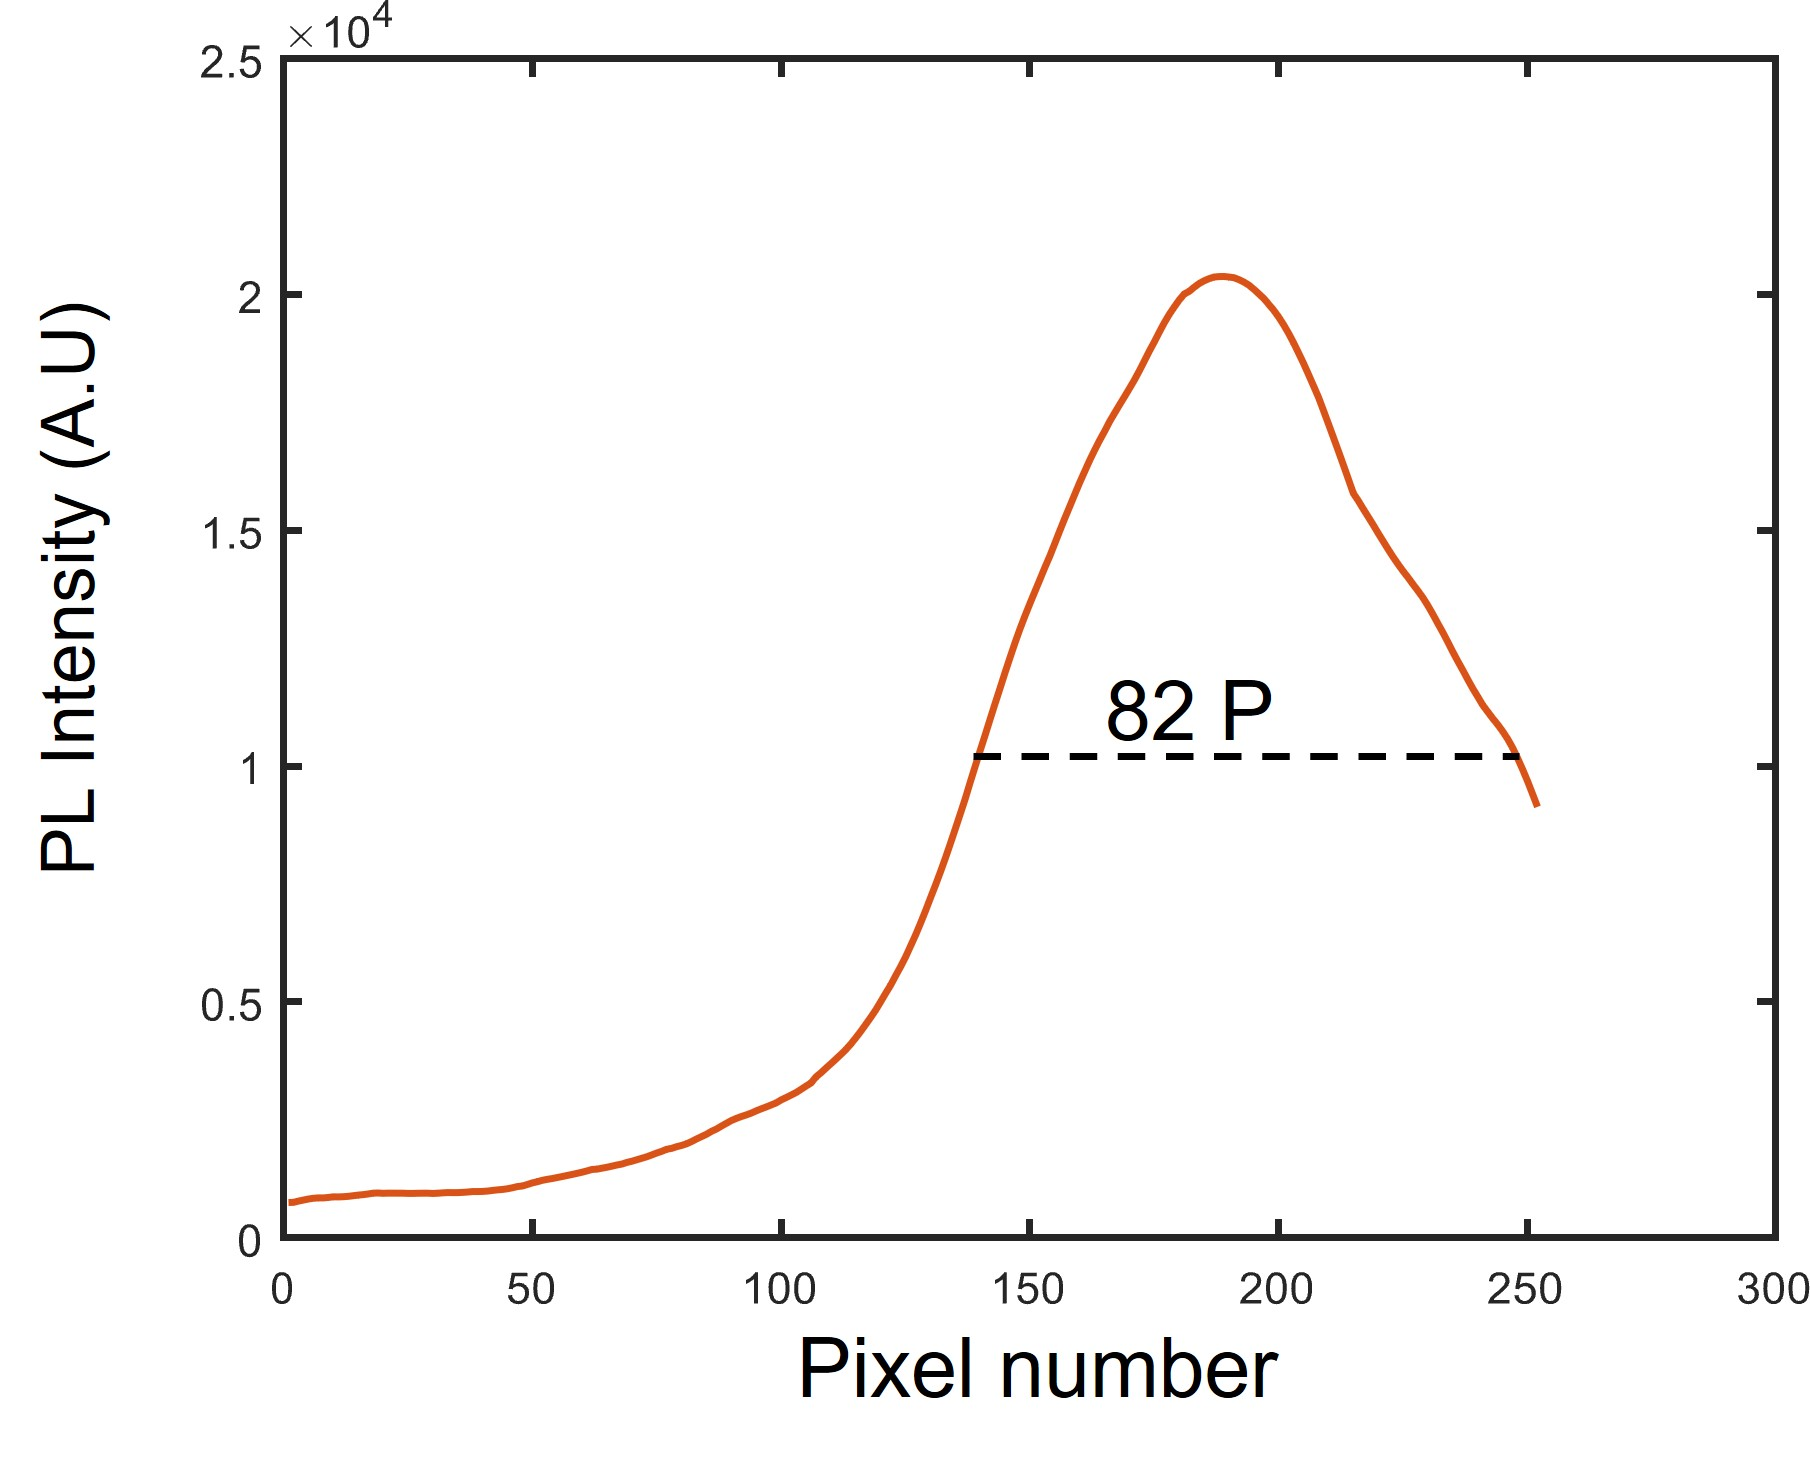} %this tells latex what graphics to include. I put my images in an 'Images' folder to aid file management, hence the Images/ before the file name. The width bit before allows you to alter the width of the image. It is also possible to use scale and equations with the text width to make it say half the text width.
    \caption{FWHM of the intensity distribution on the spectrometer camera}% this prints the caption below the figure
    \label{fig:pixel} % this internally labels the figure for future referencing.
\end{figure}
Since the pixel size is 82 microns, the FWHM is $2132 \mu m$. Knowing that the width of the spectrometer slit is $500 \mu m$, we may substitute into \ref{equation:slit}:
\begin{equation}
    \gamma_{spectrometer \: slit} = \frac{2132 \mu m \cdot 500 \mu m}{\pi \cdot (2132 \mu m)^2} \approx 0.074
\end{equation}

As for the objective system losses, we used the He:Ne laser to find the loss coefficient. Before the objective, the power was $17\mu W$, and at the end of the system (after all of the mirrors and the filters), the measured power was $6.65 \mu W$. Hence $\gamma_{system \: loses} \approx 0.3911$. 

The losses in the fiber coupling system were calculated using the same He: Ne laser. The intensity of the laser was measured before the entrance to the fiber. After the filters on the other side of the fiber, the intensity before the entrance was $17\mu W$ and $14.6\mu W$ at the end of the system (after all of the mirrors and filters).
Hence, the loss of the fiber system was  $\gamma_{fiber \: loss} \approx 0.859$.
Here again, we must find the loss due to the spectrometer slit.
\begin{equation}
 \gamma_{Fiber} = \gamma_{fiber \: system} \cdot \gamma_{fiber \: spectrometer\:slit} 
\end{equation}
Again, we will find the FWHM of the intensity distribution on the camera. 
As it can be seen, the FWHM is 43 pixels\ref{fig:pixel2}; multiplying that by the size of the pixels, we get 1118 microns.
 
\begin{figure} [H] % opens the figure environment. the '[H]' forces the image to be Here
    \centering % puts the image in the horizontal center of the page
    \includegraphics[width = 0.7\textwidth]{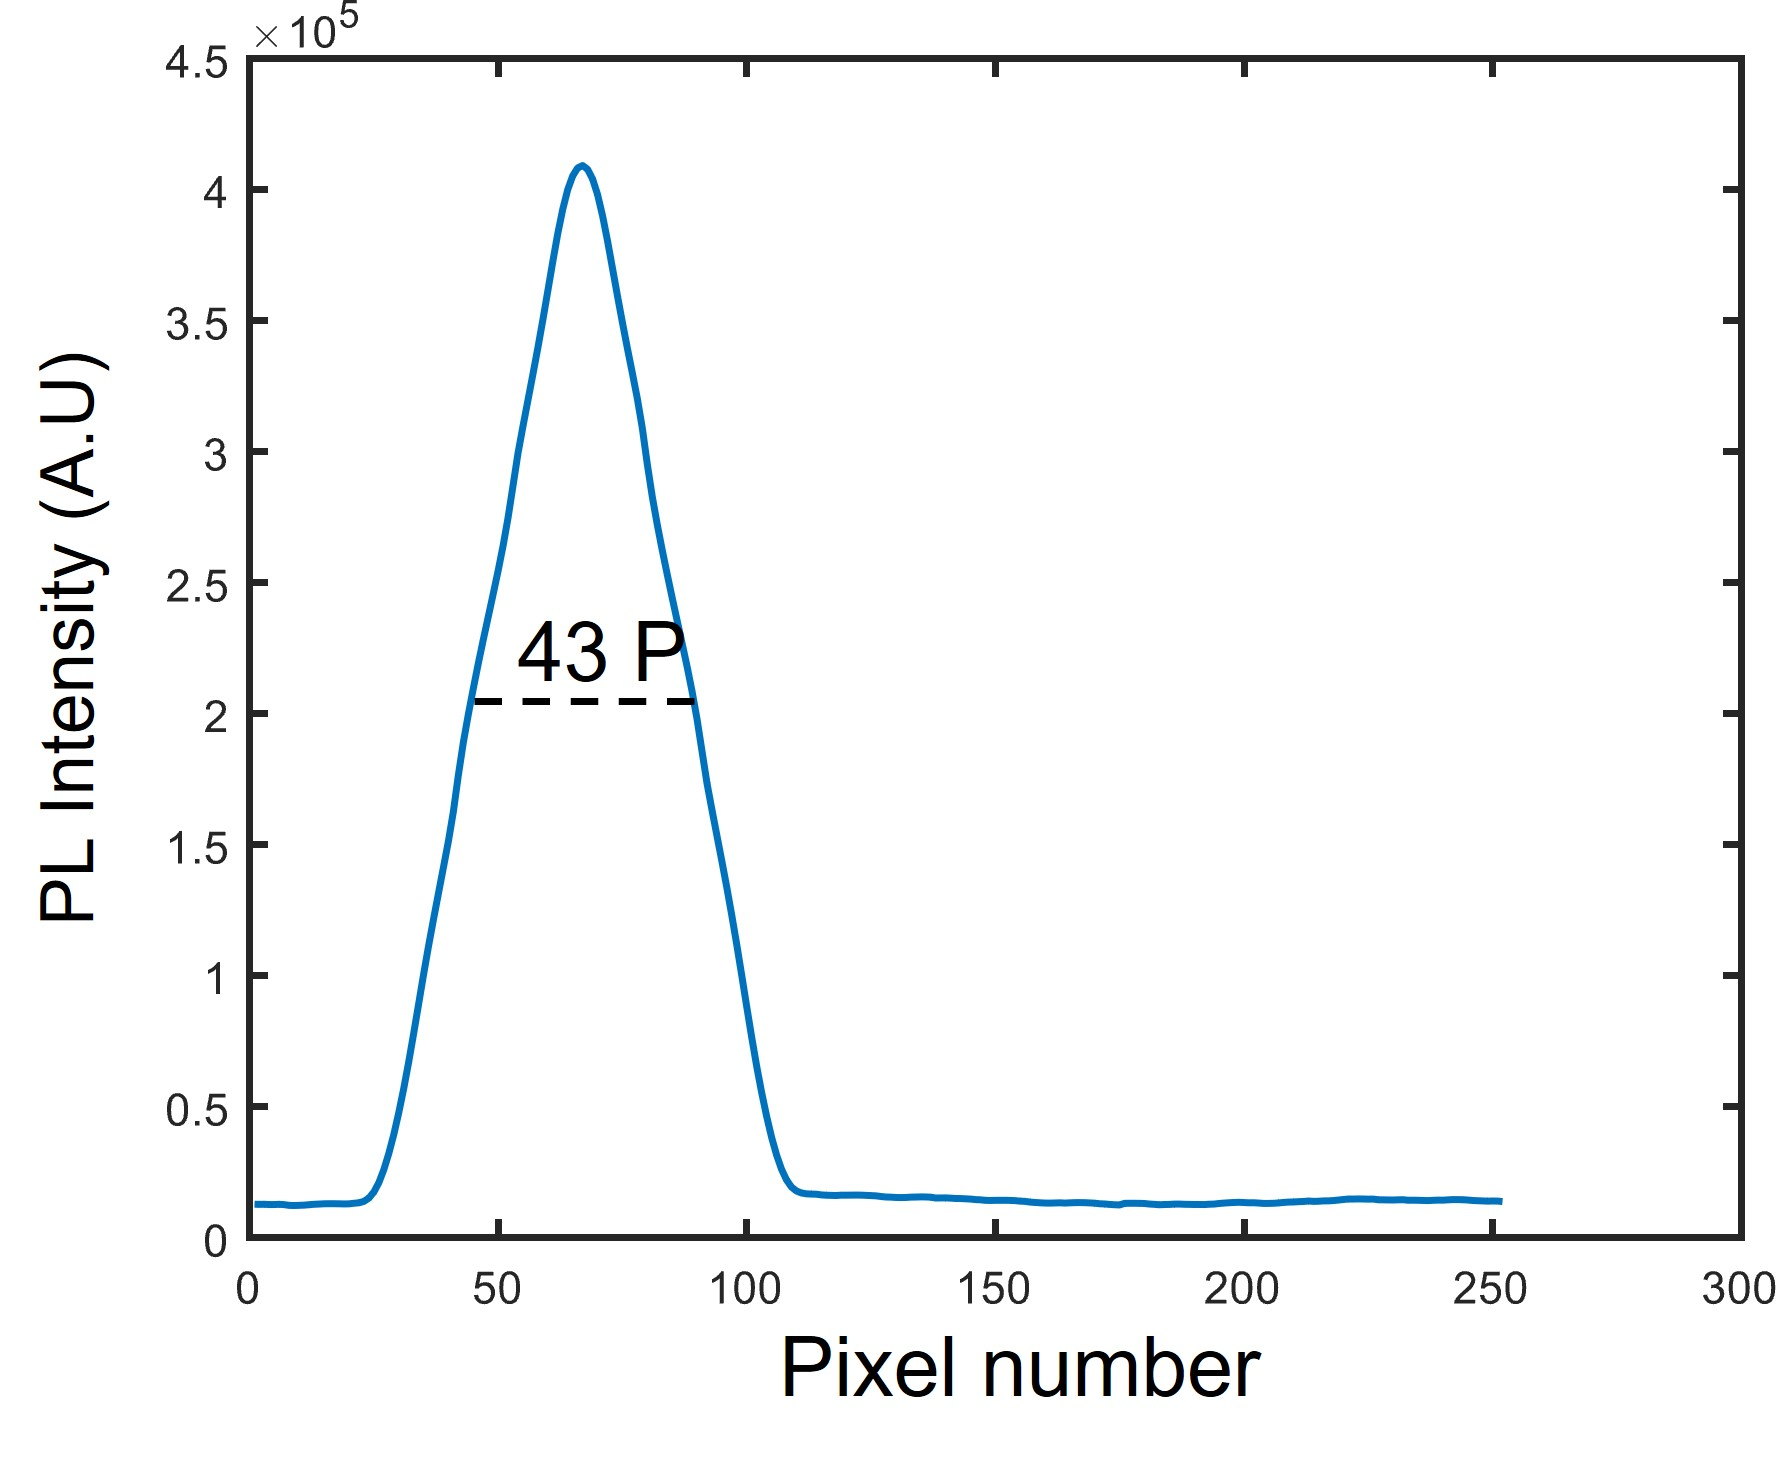} %this tells latex what graphics to include. I put my images in an 'Images' folder to aid file management, hence the Images/ before the file name. The width bit before allows you to alter the width of the image. It is also possible to use the scale as well as using equations with the textwidth to make it say half the text width.
    \caption{fiber measurement: FWHM of the intensity distribution on the spectrometer camera}% this prints the caption below the figure
    \label{fig:pixel2} % this internally labels the figure for future referencing.
\end{figure}

\begin{equation}
        \gamma_{spectrometer \: slit} = \frac{\Gamma w}{\pi \cdot \Gamma^2}
        = \frac{500 \cdot 1118}{\pi \cdot (1118)^2} = 0.1423
    \label{equation:slit2}
\end{equation}
and hence,
\begin{equation}
    \gamma_{Fiber} = 0.0854 \cdot 0.859 \approx 0.1222
\end{equation}
Now substituting all the values into the previous equation \ref{equation:fiberc}. 
\begin{equation}
    \frac{I_{Fiber\: Coupled}}{I_{0.9 NA\: objective}} \approx \frac{\int_{\lambda = 550 nm}^{\lambda = 700 nm} I_{Fiber\: Coupled}(\lambda) d\lambda \cdot 8.177}{\int_{\lambda = 550 nm}^{\lambda = 700 nm} I_{0.9 NA\: objective}(\lambda) d\lambda \cdot 34.25} = \frac{98300 \cdot 8.177}{237500 \cdot 34.25}  \approx 0.0988
    \label{equation:fiberc2}
\end{equation}
And hence the effective coupling efficiency is approximately 0.0988 \%.
\label{AppendixA}
